# Supplementary material for: Finite Sample Analysis of Minimax Offline Reinforcement Learning: Completeness, Fast Rates and First-Order Efficiency
Source: arXiv:2102.02981 source file (2022-07-24)
Supplement: Supplementary file 1 [file ape_liteature_review.tex]

%!TEX root = ../colt2021_main.tex

We briefly review several batch RL minimax estimators 

\paragraph{MIL approach }
We have defined the MIL estimators: 
\begin{align*}
  \ts  \hat J^{\MIL}_{w}&=\ts \E_n[\hat w_{\MIL}(s,a)r],\,\hat J^{\MIL}_{q}=\ts \E_{d_0}[\hat v_{\MIL}(s_0)],\hat v_{\MIL}=\hat q_{\MIL}(s,\epol),\\
     \ts \hat J^{\MIL}_{wq}&=\ts \E_n[\hat w_{\MIL}(s,a)\{r-\hat q_{\MIL}(s,a)+\gamma \hat v_{\MIL}(s')\}]+(1-\gamma)\E_{d_0}[\hat v_{\MIL}(s_0)],\\ 
     \ts  \hat w_{\MIL} &=  \ts \argmin_{w \in \Wbbb_1}\max_{q \in \Qbbb_1}\E_n[w(s,a)\{-q(s,a)+\gamma v(s')\}]+(1-\gamma)\E_{d_0}[v(s_0)]-\lambda \|-q(s,a)+\gamma v(s')\|^2_{2,n},\\
     \ts  \hat q_{\MIL}&=  \ts \argmin_{q\in \Qbbb_2}\max_{w \in \Wbbb_2}\E_n[w(s,a)\{r-q(s,a)+\gamma v(s')\}]-\lambda' \|w\|^2_{2,n},
\end{align*}
This form is the unification of many estimators. When $\lambda=0.5$, $\hat q_{\MIL}$ is modified BRM (modified Bellman Residual Minimization) \citep{antos2008learning,XieTengyang2020QASf}. When $\lambda=0$, $\hat w_{\MIL}$ is MWL in \citet{UeharaMasatoshi2019MWaQ}. When $\lambda'=0$, $\hat q_{\MIL}$ is MQL in \citet{UeharaMasatoshi2019MWaQ}. 

This unification is different from \citet{YangMengjiao2020OEvt}. In their formulation, $\lambda \|\mathcal{J}q\|^2_{2,n}$ is $\lambda \|q(s,a)\|^2_{2,n}.$ In this case, when $\lambda=1$, it is reduced to GenDICE \citep{zhang2019gendice}. At the same time, \citet{YangMengjiao2020OEvt} use more general norm rather than $L^2$-norm for stabilizers. We can also extend our analysis to this case. 

It is worthwhile to note several related estimators have been proposed in a bandit setting \citep{HirshbergDavid2019AMLE,ZhangRui2020MMRf,kallus2018balanced,WongRaymondKW2018Kcfb,ArmstrongTimothyB2017FOEa,ChernozhukovVictor2018DMLo}.

\paragraph{State-based MIL approach}

We focus on the method using action-state value functions and action-state based ratio functions. Instead, \citet{Liu2018,FengYihao2019AKLf,tang2019harnessing} proposed the state-based methods:
\begin{align*}
   \hat J^{\MIL}_{w,S} &=\E_n[\hat w_{\MIL,S}(s)\eta(s,a)r],\,    \hat J^{\MIL}_{v,S} =\E_{d_0}[\hat v_{\MIL,S}(s)],\\
     \hat J^{\MIL}_{wv,S} &=\E_n[\hat w_{\MIL,S}(s)\eta(s,a)\{r-\hat v_{\MIL,S}(s)+\gamma \hat v_{\MIL,S}(s')\}]+(1-\gamma)\E_{d_0}[\hat v_{\MIL,S}(s_0)],\\
   \hat w_{\MIL,S}&=\min_{w' \in \Wbbb_{S}}\max_{v' \in \Vbbb}\E_n[w'(s)\eta(s,a)\{-v'(s)+\gamma v'(s')\}]+(1-\gamma)\E_{d_0}[v'(s_0)]-\|-v'(s)+\gamma v'(s')\|^2_{2,n}, \\
\hat v_{\MIL,S}&=\min_{v' \in \Vbbb}\max_{w' \in \Wbbb_{S}}\E_n[w'(s)\eta(s,a)\{r-v'(s)+\gamma v'(s')\}]-\|w'\|^2_{2,n}. 
\end{align*}
The estimator $\hat J^{\MIL}_{w,S}$ corresponds to \citet{Liu2018}, $ \hat J^{\MIL}_{v,S} $ corresponds to offline version of \citet{FengYihao2019AKLf}, $\hat J^{\MIL}_{wv,S}$ corresponds to \citet{tang2019harnessing}. We can apply a similar analysis to these estimators as in the main text by some modification.
