# Supplementary material for: Finite Sample Analysis of Minimax Offline Reinforcement Learning: Completeness, Fast Rates and First-Order Efficiency
Source: arXiv:2102.02981 source file (2022-07-24)
Supplement: Supplementary file 2 [file ape_mdl.tex]

\citep{JiangNan2020MCIf,NachumOfir2019APGf} proposed minimax estimators:
\begin{align*}
      \ts \hat J^{\MDL}_{w1} &= \ts \min_{w \in \Wbbb}\max_{q \in \Qbbb}\E_n[w(s,a)\{r-q(s,a)+\gamma v(s')\}]+(1-\gamma)\E_{d_0}[v(s_0)],\\
      %J^{\MDL}_{w2} &= \ts \max_{q \in \Qbbb}\min_{w \in \Wbbb}\E_n[w(s,a)\{r-q(s,a)+\gamma v(s')\}]+(1-\gamma)\E_{d_0}[v(s_0)],\\
  \ts \hat J^{\MDL}_{q1} &=\ts \min_{q\in \Qbbb}\max_{w\in \Wbbb}\E_n[w(s,a)\{r-q(s,a)+\gamma v(s')\}]+(1-\gamma)\E_{d_0}[v(s_0)],  
\end{align*}
where $v(s)=q(s,\epol)$. We call these estimators as minimax direct learning (MDL) estimators since the estimators directly estimate $J$. 
%This estimator is analyzed in detail in \cref{ape:mdl}.

First, we give a result under $w$- and $q$- \rea.  
\begin{theorem}[Finite-sample error bound of MDL]\label{thm:generalization2}
Assume $w_{\epol}\in \Wbbb,q_{\epol}\in \Qbbb$. Letting $ \Gcal(\Wbbb,\Qbbb)=\{(s,a)\mapsto w(s,a)\{-q(s,a)+\gamma q(s',\epol)\}; w\in \Wbbb,q\in \Qbbb\}$, then, with probability $1-\delta$, 
\begin{align*}\ts
 &|\hat  J^{\MDL}-J|\lesssim \mathrm{Err}_{\MDL},\\
 &\mathrm{Err}_{\MDL}=R_{\max}\Rcal_n(\Wbbb)+\Rcal_n(\Gcal(\Wbbb,\Qbbb))+C_{\Wbbb}(R_{\max}+C_{\Qbbb})\sqrt{\log(c_0/\delta)n^{-1}},
\end{align*}
where $\hat J^{\MDL}$ is one of $\hat J^{\MDL}_{w1},\hat J^{\MDL}_{q1}$.  
\end{theorem}

This is an analogous result of \cref{thm:generalization}. In fact, the assumptions ( $w$- and $q$- \rea) and the forms of the errors are essentially the same. As explained in \cref{sec:fast_slow}, under this assumption, we cannot ensure $\hat w_{\MDL}=w_{\epol}+\op(1),\hat q_{\MDL}=q_{\epol}+\op(1)$, where $\hat w_{\MDL}$ is the argmin solution in $\hat J^{\MDL}_{w1}$ and where $\hat q_{\MDL}$ is the argmin solution in $\hat J^{\MDL}_{q1}$.  

Next, we show the sufficient conditions to ensure the convergence of $\hat w_{\MDL},\hat q_{\MDL}$. 

\begin{theorem}[Convergence rates in MDL]\label{thm:recovery2}
(1)  Suppose $w_{\epol}\in \Wbbb, C_{\xi}\Tcal'_{\gamma}(\Wbbb-w_{\epol}) \subset (\Qbbb-q_{\epol})$. Then, with $1-\delta$, $\|\hat w_{\MDL}-\Bcal'\hat w_{\MDL}\|_2\lesssim  \sqrt{C^{-1}_{\zeta}\mathrm{Err}_{\MDL}}$. 2) Suppose  $q_{\epol}\in \Qbbb,\Tcal_{\gamma}(\Qbbb-q_{\epol})\subset(\Wbbb-w_{\epol})$. Then, with $1-\delta$, $\|\hat q_{\MDL}-\Bcal\hat q_{\MDL} \|_2\lesssim   \sqrt{C^{-1}_{\zeta}\mathrm{Err}_{\MDL}}$. 
\end{theorem}

This result is a similar result to \cref{thm:recovery1} regarding MIL. However, MDL estimators require more conditions to estimate $w$, $q$-functions than MIL. The condition $w_{\epol}\in \Wbbb, C_{\xi}\Tcal'_{\gamma}(\Wbbb-w_{\epol}) = (\Bcal'-I)\Wbbb \subset (\Qbbb-q_{\epol})$ automatically implies $q_{\epol}\in \Qbbb$. Thus, both $q$-\rea and $w$-\rea are required in \cref{thm:recovery2}. On the other hand, in \cref{thm:recovery1}, what we need is just $w_{\epol}\in \Wbbb, C_{\xi}\Tcal'_{\gamma}(\Wbbb-w_{\epol}) =C_{\xi} (\Bcal'-I)\Wbbb \subset \Qbbb$, which dose not necessarily imply $q_{\epol}\in \Qbbb$. 

\begin{remark}
In \citep{JiangNan2020MCIf}, the only one-sided bound of \cref{thm:generalization2} is given.  Our result is a two-sided bound. \cref{thm:recovery2} is completely novel. 
\end{remark}
