# Supplementary material for: Finite Sample Analysis of Minimax Offline Reinforcement Learning: Completeness, Fast Rates and First-Order Efficiency
Source: arXiv:2102.02981 source file (2022-07-24)
Supplement: Supplementary file 3 [file journal_ver.tex]

%!TEX root = ../colt2021_main.tex

\begin{itemize}
    \item  Add the following in \cref{sec:preparation} "\footnote{\citet{jiang,thomas2016} give different doubly robust estimators, which include cumulative importance ratios. \citet{KallusUehara2019} gives a doubly robust estimator for time-varying MDPs. \citet{tang2019harnessing} gives a closely related doubly robust estimator. We present this estimator in \cref{ape:literature_review}.} "   \cref{sec:prepare}. 
    \item Bring back the inference stuff and the sample splitting procedure from \cref{ape:sample_splitting} to \cref{sec:efficiency}. 
    \item Write the norm theorem ($L^2$, Bellmaan residual errors) more explicitly. 
    \item Write "This types of estimators are generally called sieve estimators \citep{ChenXiaohong1998Seef}. We also present the results when using linear sieves such as polynomials and splines in \cref{ape:error}". 
    \item Bring back neural networks theorem.
    \item I need to add the following in \cref{sec:efficiency}
    \begin{remark}
Note if we assume pseudo-\comp\,instead of \comp in \cref{thm:efficiency}, the rates of $L^2$-errors are directly obtained; thus, we don't need the recovery assumption. From \cref{lem:q_completenss,lem:w_completenss}, which imply pseudo \comp hold in a tabular case, the efficiency in a tabular case is also proved from this direction.  
\end{remark}

    \item Need to add as follows in \cref{sec:preparation}: We explain a general doubly robust meta-algorithm in \citet{KallusNathan2019EBtC}, which includes MIL. Then, we introduce some operators. Doubly robust meta-algorithm was proposed in \citet{KallusNathan2019EBtC}:
\begin{align*}
   \ts  \hat J=\E_n[\hat w(s,a)\{r-\hat q(s,a)+\gamma \hat v(s')\}]+(1-\gamma)\E_{d_0}[\hat v(s_0)], \,\hat v(s)=\hat q(s,\epol),
\end{align*}
given any reasonable estimators for $\hat w(s,a)$ and $\hat q(s,a)$. MIL also takes this form, and they are regarded as specific cases. \citet{KallusNathan2019EBtC} proved that their meta algorithm is "doubly robust” in the sense that as long as $\hat w=w_{\epol}+\op(1)$ or $\hat q=q_{\epol}+\op(1)$, then $\hat J= J(\epol)+\op(1)$. However, this result does \emph{not} exactly show "genuine double robustness” since we need more essential conditions beyond the realizability $w_{\epol}\in \Wbbb,q_{\epol}\in\Qbbb$ to state $\hat w=w_{\epol}+\op(1)$ or $\hat q=q_{\epol}+\op(1)$. For example, we need completeness regarding $\Qbbb$ to ensure $\hat q=q_{\epol}+\op(1)$ in FQI \citep{munos2008finite}. On the other hand, in a bandit setting, the \rea is enough to ensure $\hat q=q_{\epol}+\op(1)$. The same argument is applied to  $\hat w=w_{\epol}+\op(1)$. This describes difficulties of OPE in RL comparing to a bandit setting. In our work, the goal is providing genuine sufficient conditions to estimate $J(\epol),w_{\epol},q_{\epol}$. 
\item \paragraph{DICE methods}\masa{ongoing}

\txie{Comparison with DICE etc. notations will be fixed later for consistency}

We now summarize the different methods of estimating Q-function and weight function. We present our comparison using the matrix formulation, where $q_\pi$ denotes the $|\Scal| \Acal| \times 1$ vector of Q-function and $w_\pi$ and $d_\pi$ denote the $1 \times |\Scal| \Acal|$ vectors of weight function and density function. Also let $\Pcal^\pi$ be an $|\Scal| \Acal| \times |\Scal| \Acal|$ matrix, where its $\Pcal^\pi_{s'a',sa} \coloneqq \Pr(s_{t + 1} = s', a_{t + 1} = a' | s_{t} = s, a_{t} = a, a_{t + 1} \sim \pi(\cdot|s_{t + 1}))$. We also use $D_\mu$ to denote an $|\Scal| \Acal| \times |\Scal| \Acal|$ diagonal matrix whose $s,a$-th diagonal element is $\mu(s,a)$. 

Using this matrix formulation, we can write the Bellman function of $q_\pi$ and $d_\pi$ as follows, which is the first principle of estimating Q-function and weight function over all these methods,
\begin{align}
% \label{eq:dpiBE}
d_\pi (I - \gamma \Pcal^\pi) = &~ (1 - \gamma) d_0^\pi,  \tag*{[Bellman equation of $d_\pi$]}
\\
% \label{eq:qBE}
(I - \gamma \Pcal^\pi) q_\pi = &~ R^\pi.  \qquad  \tag*{[Bellman equation of $q_\pi$]}
\end{align}
When considering the the weight function $w_\pi$ ($\coloneqq d_\pi / \mu$), we have
\begin{align}
w_\pi \Dcal_\mu (I - \gamma \Pcal^\pi) = &~ (1 - \gamma) d_0^\pi.  \quad  \tag*{[Bellman equation of $w_\pi$]}
\end{align}

\paragraph{DualDICE}
DualDICE \citep{ChowYinlam2019DBEo} calculates $w_\pi$ by designing a objective whose gradient is connected with the Bellman residual on $w_\pi$. That is, if we define $\nu \coloneqq (I - \gamma \Pcal^\pi)^{-1} w_\pi^\top$, then we can rewrite the Bellman equation of $w_\pi$ as
\begin{align*}
\nu^\top (I - \gamma \Pcal^\pi)^\top \Dcal_\mu (I - \gamma \Pcal^\pi) = &~ (1 - \gamma) d_0^\pi.
\end{align*}
Note that, the equality holds if and only if $\nu$ is the stationary point of the following objective (gradient equals to zero), which is exactly the objective used in \citep{ChowYinlam2019DBEo},
\begin{align*}
\Lcal_{\text{DualDICE}}(\nu) \coloneqq \frac{1}{2} \nu^\top (I - \gamma \Pcal^\pi)^\top \Dcal_\mu (I - \gamma \Pcal^\pi) \nu - (1 - \gamma) d_0^\pi \nu.
\end{align*}

\paragraph{GenDICE, GradientDICE, Policy-Evaluation Variant of SBEED or MSBO}
This line of methods minimize the Bellman residual of $q_\pi$ or $w_\pi$ using Fenchel duality. Note that, although SBEED and MSBO are designed for policy optimization, they can be adopted to policy evaluation directly by changing the Bellman optimality operator to the Bellman operator.

The objective of GenDICE \citep{zhang2019gendice} is built over $D_\phi(w_\pi \Dcal_\mu \| \gamma w_\pi \Dcal_\mu \Pcal^\pi + (1 - \gamma) d_0^\pi)$, where $D_\phi$ is the $f$-divergence associated with a convex function $\phi$.

GradientDICE \citep{gradientdice20zhang} extends GenDICE using a linear parametrization, which addresses the convergence issue in GenDICE. GradientDICE eliminates the nonlinearity in GenDICE by replacing the use of $f$-divergence GenDICE to an objective of a weighted 2-norm, and proposing an objective based on $\|w_\pi \Dcal_\mu - \gamma w_\pi \Dcal_\mu \Pcal^\pi - (1 - \gamma) d_0^\pi\|_{\Dcal_\mu^{-1}}$ (plus the regularization term).

SBEED \citep{dai2018}

MSBO \citep{XieTengyang2020QASf}

\paragraph{MWL, MQL \citep{UeharaMasatoshi2019MWaQ}}

\end{itemize}
