# Supplementary material for: Finite Sample Analysis of Minimax Offline Reinforcement Learning: Completeness, Fast Rates and First-Order Efficiency
Source: arXiv:2102.02981 source file (2022-07-24)
Supplement: Supplementary file 4 [file ape_analysis_mdl.tex]

%!TEX root = ../colt2021_main.tex

We analyze MDL approaches. First, we give an analogues result as \cref{thm:generalization}. In \citet{JiangNan2020MCIf}, the only one-sided bound is given.

\begin{theorem}[Finite sample bound of MDL]\label{thm:generalization2}
Assume $w_{\epol}\in \Wbbb,q_{\epol}\in \Qbbb$. Letting $ \Gcal(\Wbbb,\Qbbb)=\{(s,a)\mapsto w(s,a)\{-q(s,a)+\gamma q(s',\epol)\}; w\in \Wbbb,q\in \Qbbb\}$, then, with probability $1-\delta$, 
\begin{align*}\ts
 &|\hat  J^{\MDL}-J|\lesssim \mathrm{Err}_{\MDL},\,\mathrm{Err}_{\MDL}=R_{\max}\Rcal_n(\Wbbb)+\Rcal_n(\Gcal(\Wbbb,\Qbbb))+C_{\Wbbb}(R_{\max}+C_{\Qbbb})\sqrt{\log(c_0/\delta)n^{-1}}.  
\end{align*}
where $\hat J^{\MDL}$ is one of $\hat J^{\MDL}_{w1},\hat J^{\MDL}_{q1}$.  
\end{theorem}

Next, we give an analogues result as \cref{thm:recovery1}.

\begin{theorem}[Convergence rates in MDL]\label{thm:recovery2}
(1)  Suppose $w_{\epol}\in \Wbbb, C_{\zeta}\Tcal'_{\gamma}(\Wbbb-w_{\epol}) \subset (\Qbbb-q_{\epol})$. Then, with $1-\delta$, $\|\hat w_{\MDL}-\Bcal'\hat w_{\MDL}\|_2\lesssim  \sqrt{C^{-1}_{\zeta}\mathrm{Err}_{\MDL}}$, where $\hat w^{\MDL}$ is the argmin solution in $\hat J^{\MDL}_{w1}$. 2) Suppose  $q_{\epol}\in \Qbbb,\Tcal_{\gamma}(\Qbbb-q_{\epol})\subset(\Wbbb-w_{\epol})$. Then, with $1-\delta$, $\|\hat q_{\MDL}-\Bcal\hat q_{\MDL} \|_2\lesssim   \sqrt{C^{-1}_{\zeta}\mathrm{Err}_{\MDL}}$, where $\hat q^{\MDL}$ is the argmin solution in $\hat J^{\MDL}_{q1}$. 
\end{theorem}

MDL requires more conditions to estimate $w$, $q$-functions than MIL. In fact, $w_{\epol}\in \Wbbb, (\Bcal'-I)\Wbbb \subset (\Qbbb-q_{\epol})$ automatically implies $q_{\epol}\in \Qbbb$. Thus, both $q$-\rea and $w$-\rea are required.
