# Supplementary material for: Finite Sample Analysis of Minimax Offline Reinforcement Learning: Completeness, Fast Rates and First-Order Efficiency
Source: arXiv:2102.02981 source file (2022-07-24)
Supplement: Supplementary file 6 [file ape_sample_splitting.tex]

%!TEX root = ../colt2021_main.tex


We explain the sample-splitting procedure. This technique is traditionally used to analyze the plug-in type estimators such as the functional of nonparametric estimators \citep{1987CEot,VaartA.W.vander1998As}. Recently, it has also been used a lot in the context of causal inference \citep{ChernozhukovVictor2018Dmlf,FosterDylanJ.2019OSL}. In an RL context, \citet{KallusUehara2019} apply this technique to OPE. By sample splitting, we can easily analyze the terms called stochastic equicontinutiy terms. 


Let be $\phi(s,a,r,s';w,q)\coloneqq w(s,a)\{r-q(s,a)+\gamma q(s',\epol)\}+\E_{d_0}[q(s_0,\epol)]$. 
\begin{enumerate}
    \item Split the whole sample into half as $\Dcal_0$, $\Dcal_1$. 
    \item Construct estimators $\hat w^{\MIL}_0,\hat q^{\MIL}_0$ using $\Dcal_0$, and define $\hat J_0=\frac{2}{n}\sum_{i\in \Dcal_1}\phi(s^i,a^i,r^i,s'^i;\hat w^{\MIL}_0,\hat q^{\MIL}_0)$.
    \item Construct estimators $\hat w^{\MIL}_1,\hat q^{\MIL}_1$ using $\Dcal_1$, and define $\hat J_1=\frac{2}{n}\sum_{i\in \Dcal_0}\phi(s^i,a^i,r^i,s'^i;\hat w^{\MIL}_1,\hat q^{\MIL}_1)$. 
    \item Redefine $\hat J_{wq}=0.5(\hat J_0+\hat J_1)$. 
\end{enumerate}

%\paragraph{Inference}\masa{add the proof later}
%We can do inference from the following corollary. The testing based on the efficient estimator is “locally uniformly most powerful" \citep[Theoreme 25.44]{VaartA.W.vander1998As}. 
%\begin{corollary}
%Assume the conditions in \cref{thm:efficiency}. Suppose $\eta_w\eta_q=o(n^{-1/2})$. Then, 
%\begin{align*}
%  \ts  \sqrt{n}(\hat J^{\MIL}_{wq}-J)\xrightarrow{d}\Ncal(0,\E[w^2_{\epol}(s,a)\{r-q(s,a)+q(s',\epol)\}^2]). 
%\end{align*}
%\end{corollary}
